# Supplementary material for: Twist, Don't Tilt: Trajectory-Exact Constrained Decoding for Masked Diffusion Models
Source: arXiv:2609.35609 source file (2026-09-28)
Supplement: Supplementary file 1 [file dfa_states_swarm-macros.tex]

%% Auto-generated by cedar.experiments.dfa_sizes.plot_dfa_sizes
\newcommand{\dfaStatesN}{94\xspace}
\newcommand{\dfaStatesMin}{34\xspace}
\newcommand{\dfaStatesMean}{188\xspace}
\newcommand{\dfaStatesMax}{625\xspace}
